# Supplementary material for: Molecular Generation with Recurrent Neural Networks (RNNs)
Source: arXiv:1705.04612 ancillary file (2017-05-17)
Supplement: Supplementary file 1 [file Supplementary_information.pdf]

Supplementary information for

**Molecular Generation with Recurrent Neural Networks (RNNs)**

Esben Jannik Bjerrum1,*Richard Threlfall2

1) Wildcard Pharmaceutical Consulting, Frødings Allé 41, 2860 Søborg, Denmark.
2) Wiley-VCH, Boschstrasse 12, 69469 Weinheim, Germany
*) esben@wildcardconsulting.dk

arXiv:1705.04612

| Group | SMILES | SA Score | No. of synthesis routes | Steps min (from most advanced CASM) | Steps max (from CASM <$1000) | Yield % | Cost of SMs US$/100g | Comments |
|---|---|---|---|---|---|---|---|---|
| easy 1 | CN1CCC(CNC(=O)NCCNC(=O)c2ccccc2)CC1 | 1.9372 | 20 | 2 | 2 | 52 | 1094 | |
| easy 2 | O=C(O)Cc1ccc(NS(=O)(=O)c2c(F)cccc2F)cc1 | 1.9372 | 23 | 1 | 1 | 73 | 1112 | |
| easy 3 | CCN(Cc1ccccc1)c1ccc(N)cc1C(=O)O | 1.9373 | 34 | 1 | 1 | 70 | 184 | |
| easy 4 | COc1ccc(NC(=O)c2ccco2)cc1I | 1.9374 | 39 | 1 | 2 | 58 | 273 | |
| easy 5 | O=C(NCCc1ccccc1)c1ccc(F)c(S(=O)(=O)N2CCCCCCC2)c1 | 1.9375 | 20 | 2 | 3 | 52 | 2344 | |
| easy 6 | CN(C)C(=O)Nc1ccc(CNC(=O)c2ccc3c(c2)CCC3)cc1 | 1.9375 | 20 | 2 | 4 | 29 | 1256 | |
| medium 1 | CCN(C(=O)Nc1cccc(CCN2CCCC2)c1)C(C)c1ccc(C#N)cc1 | 2.6859 | 39 | 2 | 3 | 33 | 1907 | |
| medium 2 | CCC(CC)(c1ccccc1)c1nc2c(c(=O)[nH]1)CCCC2 | 2.6859 | 27 | 3 | 4 | 25 | 37 | |
| medium 3 | CC(NC(=O)CCc1nncn1-c1ccccc1)c1ccc(C(F)(F)F)cc1 | 2.6860 | 31 | 3 | 4 | 34 | 2437 | |
| medium 4 | CN1CCN(C(CNC(=O)c2cccs2)c2ccco2)CC1 | 2.6860 | 63 | 2 | 2 | 56 | 1012 | 2nd ranked route |
| medium 5 | CCc1ccc(C(C)(C)CNC(=O)N2CCCC(N(C)C)CC2)cc1 | 2.6858 | 39 | 4 | 6 | 31 | 1697 | |
| medium 6 | CN(CC1CCCN1C)C(=O)c1cccc(OCc2c(F)cccc2Cl)c1 | 2.6858 | 41 | 2 | 3 | 32 | 3055 | |
| hard 1 | CC1CCC(C(=O)O)C(N2CCOC(C)(C)C2)C1 | 3.6575 | 43 | 2 | 4 | 31 | 1028 | |
| hard 2 | N#Cc1cc(Cl)cc2c1C1C=CCC1C(c1ccc(Br)cc1)N2 | 3.6576 | 63 | 4 | 5 | 23 | 2509 | |
| hard 3 | COCC(C)(NC(=O)c1nnn[nH]1)C(=O)OC | 3.6575 | 23 | 4 | 4 | 34 | 80 | |
| hard 4 | Cc1nn(CC(C)C)cc1C(C)NCC(C)(O)c1ccsc1 | 3.6576 | 37 | 3 | 5 | 20 | 195 | |
| hard 5 | CC(C)OC(=O)C1=C(Nc2ccc(Cl)c(C(=O)O)c2OC(C)C)Nc2nnnn2C1c1ccccc | 3.6574 | | >10 | >10 | | | |
| hard 6 | CC(C(=O)N1C(C)CCCC1C)N(C)C1CCC(C)(C)CC1 | 3.6578 | 28 | 3 | 4 | 26 | 153 | |
| hard 7 | Cc1ccc(C(C)n2cc(C(=O)N3CCOCC3C3CC3)nn2)o1 | 3.6578 | 86 | 5 | 6 | 22 | 2624 | common rules, 4 steps |
| hard 8 | Cc1cc(C(N)c2cncn2C2CC2)sc1Br | 3.6573 | 22 | 4 | 4 | 17 | 4599 | common rules, 4 steps |
| hard 9 | CCCNC1(C#N)CCCC1CCSc1ccc(Br)cc1 | 3.6571 | 35 | 3 | 3 | 36 | 2550 | |
| hardest | CCCC(CN)C1(O)CC2CCN1CC21C=CCC1 | 6.07 | | >10 | >10 | | | |

Yield and SM costs based on synthesis in column E

| Averages | Possible Selectivity Issues | SA Score | No. of synthesis routes | Steps min (from most advanced CASM) | Steps max (from CASM <$1000) | Yield % | Cost of SMs US$/100g |
|---|---|---|---|---|---|---|---|
| Easy | 0/6 | 1.9 | 26.0 | 1.5 | 2.2 | 55.7 | 1043.8 |
| Medium | 1/6 | 2.7 | 40.0 | 2.7 | 3.7 | 35.2 | 1690.8 |
| Hard | 4/9 | 3.7 | 42.1 | 3.5 | 4.4 | 26.1 | 1717.3 |

Yellow Marking:

Estimated possibility of selectivity issues in steps for top ranked route

| | |
|---|---|
| Description | based on the full routes, which corresponds to the number of steps in column E. Column D is the shortest route from the most advanced commercially available starting material that doesn’t meet the $1000 price criterion. Where a route is marked in yellow, this means that there may be a possibility of selectivity issues with one or more reactions in the top-ranked route. In the case of medium 4, the second-ranked route is included because the first contained a transformation that, seem very unlikely to work without protecting groups, which would add more steps. Compounds hard 7 and hard 8 required 4 steps with common reaction rules to solve to commercially available starting materials. Compounds hard 5 and hardest could not be solved on any of the settings up to and including 4 steps with rare rules after three rounds of analysis. The starting material compounds found in the first round were resubmitted for two further analyses and did not reach a commercially available starting material. |
